# Supplementary material for: HYPE: A Benchmark for Human eYe Perceptual Evaluation of Generative Models
Source: arXiv:1904.01121 source file (2019-10-31)
Supplement: Supplementary file 1 [file 08_appendix.tex]

\allowdisplaybreaks
\clearpage

\onecolumn
\section*{Appendix}

\subsection*{A. Confidence Intervals}
\label{sec:appendix-D}

\begin{table}[h]
\centering
\caption{Full bootstrapped 95\% confidence intervals from \systeminf}.
\begin{tabular}{lrrlr}
\toprule
    Model &   Std &   Deception Rate & 95\% CI &  Number of Evaluators \\
\midrule
  WGAN-GP &  0.84 &   3.79 &    2.29--5.52 &                    10 \\
  WGAN-GP &  0.69 &   3.78 &     2.5--5.21 &                    15 \\
  WGAN-GP &  0.61 &   3.78 &    2.66--5.05 &                    20 \\
  WGAN-GP &  0.54 &   3.79 &    2.79--4.92 &                    25 \\
  WGAN-GP &  0.49 &   3.78 &    2.85--4.76 &                    30 \\
  WGAN-GP &  0.45 &   3.78 &     2.95--4.7 &                    35 \\
  WGAN-GP &  0.43 &   3.79 &    2.97--4.64 &                    40 \\
    BEGAN &  2.65 &  10.04 &   5.73--15.83 &                    10 \\
    BEGAN &  2.20 &   9.99 &   6.18--14.72 &                    15 \\
    BEGAN &  1.86 &   9.97 &   6.72--13.91 &                    20 \\
    BEGAN &  1.67 &  10.01 &   7.04--13.62 &                    25 \\
    BEGAN &  1.55 &   9.99 &    7.26--13.3 &                    30 \\
    BEGAN &  1.42 &  10.00 &   7.44--12.95 &                    35 \\
    BEGAN &  1.33 &  10.00 &    7.6--12.76 &                    40 \\
   ProGAN &  1.53 &  40.30 &  37.19--43.23 &                    10 \\
   ProGAN &  1.24 &  40.28 &  37.78--42.57 &                    15 \\
   ProGAN &  1.08 &  40.29 &   38.12--42.4 &                    20 \\
   ProGAN &  0.97 &  40.27 &  38.38--42.12 &                    25 \\
   ProGAN &  0.87 &  40.29 &  38.54--41.94 &                    30 \\
   ProGAN &  0.83 &  40.27 &   38.6--41.87 &                    35 \\
   ProGAN &  0.76 &  40.29 &  38.75--41.74 &                    40 \\
 StyleGAN &  2.19 &  50.66 &   46.35--54.9 &                    10 \\
 StyleGAN &  1.79 &  50.68 &  47.08--54.17 &                    15 \\
 StyleGAN &  1.57 &  50.67 &    47.6--53.7 &                    20 \\
 StyleGAN &  1.38 &  50.65 &  47.92--53.29 &                    25 \\
 StyleGAN &  1.27 &  50.66 &  48.16--53.16 &                    30 \\
 StyleGAN &  1.16 &  50.68 &  48.39--52.95 &                    35 \\
 StyleGAN &  1.09 &  50.64 &  48.49--52.71 &                    40 \\
   \trunc &  4.21 &  27.59 &    19.7--35.9 &                    10 \\
   \trunc &  3.46 &  27.60 &  20.93--34.53 &                    15 \\
   \trunc &  2.95 &  27.65 &   22.0--33.55 &                    20 \\
   \trunc &  2.69 &  27.58 &  22.44--32.96 &                    25 \\
   \trunc &  2.44 &  27.60 &   22.9--32.43 &                    30 \\
   \trunc &  2.25 &  27.64 &  23.34--32.17 &                    35 \\
   \trunc &  2.13 &  27.62 &   23.5--31.87 &                    40 \\
 \notrunc &  3.04 &  19.06 &    13.1--25.1 &                    10 \\
 \notrunc &  2.50 &  19.02 &  14.13--23.93 &                    15 \\
 \notrunc &  2.17 &  18.99 &  14.75--23.25 &                    20 \\
 \notrunc &  1.96 &  18.96 &  15.08--22.84 &                    25 \\
 \notrunc &  1.77 &  18.95 &   15.5--22.43 &                    30 \\
 \notrunc &  1.62 &  18.98 &   15.8--22.23 &                    35 \\
 \notrunc &  1.52 &  18.98 &   16.0--22.05 &                    40 \\
\bottomrule
\end{tabular}
\end{table}

\begin{table}[h]
\centering
\caption{Full bootstrapped 95\% confidence intervals from \systemstair}.
\begin{tabular}{lrrlr}
\toprule
    Model &    Std &    Mean &         95\% CI &  Number of Evaluators \\
\midrule
  WGAN-GP &   0.00 &  100.00 &    100.0--100.0 &                    10 \\
  WGAN-GP &   0.00 &  100.00 &    100.0--100.0 &                    15 \\
  WGAN-GP &   0.00 &  100.00 &    100.0--100.0 &                    20 \\
  WGAN-GP &   0.00 &  100.00 &    100.0--100.0 &                    25 \\
  WGAN-GP &   0.00 &  100.00 &    100.0--100.0 &                    30 \\
    BEGAN &  12.50 &  107.28 &    100.0--100.0 &                    10 \\
    BEGAN &  10.08 &  107.33 &    100.0--100.0 &                    15 \\
    BEGAN &   8.85 &  107.41 &    100.0--100.0 &                    20 \\
    BEGAN &   7.86 &  107.34 &    100.0--108.8 &                    25 \\
    BEGAN &   7.06 &  107.24 &   100.0--107.33 &                    30 \\
   \trunc &  52.29 &  364.88 &    243.0--365.0 &                    10 \\
   \trunc &  42.95 &  365.84 &    266.0--366.0 &                    15 \\
   \trunc &  37.54 &  365.35 &    279.0--365.0 &                    20 \\
   \trunc &  33.21 &  365.33 &    288.0--365.2 &                    25 \\
   \trunc &  30.34 &  365.59 &   295.67--365.0 &                    30 \\
   \trunc &  28.12 &  365.20 &  301.43--364.57 &                    35 \\
   \trunc &  26.22 &  365.60 &   305.5--365.25 &                    40 \\
 \notrunc &  49.28 &  242.99 &    143.0--239.0 &                    10 \\
 \notrunc &  40.33 &  243.07 &  157.33--240.67 &                    15 \\
 \notrunc &  34.75 &  243.71 &    171.5--241.5 &                    20 \\
 \notrunc &  31.31 &  243.16 &    176.4--241.6 &                    25 \\
 \notrunc &  28.32 &  243.33 &   182.0--241.67 &                    30 \\
 \notrunc &  26.19 &  243.19 &   187.14--242.0 &                    35 \\
 \notrunc &  24.37 &  243.03 &  191.25--241.75 &                    40 \\
   ProGAN &  51.03 &  335.55 &    221.0--335.0 &                    10 \\
   ProGAN &  41.97 &  336.14 &  241.33--335.33 &                    15 \\
   ProGAN &  36.31 &  335.38 &    252.0--335.0 &                    20 \\
   ProGAN &  32.25 &  336.05 &    262.4--335.2 &                    25 \\
   ProGAN &  29.72 &  335.17 &   268.0--334.67 &                    30 \\
 StyleGAN &  56.36 &  368.82 &    237.0--368.0 &                    10 \\
 StyleGAN &  46.07 &  369.46 &   262.0--368.67 &                    15 \\
 StyleGAN &  39.94 &  368.86 &    277.0--368.5 &                    20 \\
 StyleGAN &  35.66 &  368.66 &    285.2--368.4 &                    25 \\
 StyleGAN &  32.53 &  368.82 &  295.33--368.33 &                    30 \\
\bottomrule
\end{tabular}
\end{table}
